# Supplementary material for: MegaScale-Omni: A Hyper-Scale, Workload-Resilient System for MultiModal LLM Training in Production
Source: arXiv:2605.08962 source file (2026-05-09)
Supplement: Supplementary file 1 [file appendix.tex]

\section{Hello World}
%\subsection{Hello World}
